# Supplementary material for: Rethinking BPS: A Utility-Based Evaluation Framework
Source: arXiv:2505.22316 source file (2025-05-28)
Supplement: Supplementary file 1 [file 07_Appendix.tex]

\newpage
\appendix

\section{Proofs and Remarks}
% the \\ insures the section title is centered below the phrase: AppendixA

\setcounter{theorem}{0}
\begin{theorem}\label{prop_w1}
The Wasserstein-1 distance between two empirical distributions $\mathbf{P}$ and $\mathbf{Q}$ with samples $\{X_i\}$ and $\{Y_i\}$ of  size $n$ in $\mathbb{R}^1$ can be written as:
\begin{equation}
W_1(\mathbf{P}, \mathbf{Q}) 
\;=\; 
\frac{1}{n} \sum_{i=1}^n \bigl| X_{(i)} - Y_{(i)} \bigr|, \label{PropEMDeq}
\end{equation}
where $X_{(i)}$ and $Y_{(i)}$ denote the $i$-th order statistics (sorted samples).
\end{theorem}

\begin{proof}
    The proof chiefly relies on the work of \citeA{villani2003topics_A}. Given that $\mathbf{P}$ and $\mathbf{Q}$ are discrete, real-valued random variables, we are able to reduce the Optimal Transport Problem to the following structure: 
    \begin{equation}
        W_1(\mathbf{P}, \mathbf{Q}) = \inf\left\{ \frac{1}{n}\sum_i |X_i - Y_{\sigma(i)}|: \hspace{0.1cm} \sigma \in S_n \right\}. \label{PropEMDGeneralEQ}
    \end{equation}
    Here, $S_n$ describes the space of permutations for $n-$tuples. In the following, we want to show that \autoref{PropEMDGeneralEQ} is solved by \autoref{PropEMDeq}. Without loss of generality, let $X_1^{\downarrow}, X_2^{\downarrow}, \dots, X_n^{\downarrow}$ describe the \textit{descending} ordering of $(X_i)_{i=1}^n$, i.e., $X_i^{\downarrow} \geq X_{i+1}^{\downarrow}$, $i=1,\dots, n-1$. Next, let 
    \begin{equation}
        f_i: \mathbb{R} \longrightarrow \mathbb{R}, \quad x\longmapsto \lvert X_i^{\downarrow} - x \rvert.
    \end{equation}
    One may quickly verify that $f_{i+1} - f_i$ is a non-decreasing function for any $i \in \{1, \dots, n-1\}$. Now, utilizing the result of Problem 5.4. in \citeA{cauchyschwarzmc_A}, we obtain that for any permutation $\sigma \in S_n$, \begin{equation}
        \sum_{i=1}^n f_i(Y_i^{\downarrow}) = \sum_{i=1}^n \lvert X_i^{\downarrow} - Y_i^{\downarrow}\rvert\leq \sum_{i=1}^n f_i(Y_{\sigma(i)}^{\downarrow}).
    \end{equation} 
    Due to commutativity of the sum, the actual ordering along $i$ becomes irrelevant as long as the pairings remain intact. This concludes our assertion. \qed
\end{proof}

\begin{remark}
On a side note, in \citeA{chapela2025_A}, two conceptual variants to measuring the distance between two time series sequences are proposed. The first one requires that the number of observations (i.e. the total mass) of both time series is equal. They are then transformed into histograms of relative probabilities via normalization and the W-1 distance is calculated. The second one does not assume equal total masses and is applied '''directly''' to the frequency-histograms (EMD). We will, however, only focus on the Wasserstein distance when referring to this step. Note that in the first case, the EMD would yield an identical result (cf. \citeA{mallow_emd_A}). Moreover, as the authors of \citeA{chapela2025_A} conclude, in case of much total mass and/or approx. similar sequence-lengths, the computation of W1 is more efficient and leads to similar results compared to EMD.  
\end{remark}

\section{Additional Results}
\subsection{Experiment 1}
We provide a few more details about the \emph{Loan Application} process here.
The process consists of 12 activities, starting with \emph{Check application form completeness}. It includes one loop, a parallel branch of three activities, three exclusive split gateways, and three possible end points: \emph{Approve application}, \emph{Reject application}, and \emph{Cancel application}. The process is executed by 19 distinct resources.

We look at different modifications of the ground truth log to assess the validity of our framework:
\begin{itemize}[noitemsep, topsep=0pt]
    \item Loan$_{SEQ}$: arranging the three parallel activities \emph{Appraise property}, \emph{Check credit history}, and \emph{AML check} as a sequence. 
    \item Loan$_{S{\text -}G}$: altering, on top of Loan$_{SEQ}$, the branching probabilities.
    \item Loan$_{RC}$: halving the available resources. 
    \item Loan$_{EXT}$: adding extraneous waiting time to delay the start of activities. 
    \item Loan$_{DUR}$: increasing the duration of the activities of the process.
    \item Loan$_{CAL}$: changing resource working schedules from 9am-5pm to 2pm-10pm.
    \item Loan$_{ARR}$: increase the rate of case arrivals from 30 minutes to 15 minutes on average.
\end{itemize}

\subsection{Experiment 2}
In addition to our aggregated results provided in the main paper, we report the individual results of the LSTM and Transformer approaches here as well in \autoref{tab:results_LSTM} and \autoref{tab:results_transformer}.

% First full-page table without page number/style
\vspace*{\fill}
\begin{table}[htbp]
    \centering
    \caption{Performance of LSTM model on real and simulated data. Each table entry shows the average performance over 10 runs, with the standard deviation in parentheses.}
    \begin{tabular}{clrrrrr}
        \toprule
        Log & Data & NAP & NRP & NPP(min) & NWP(hour) & RTP(day) \\
        \midrule
        \multirow{4}{*}{\rotatebox{90}{P2P}} & real & 0.84 (0.03) & 0.83 (0.01) & 70.24 (15.51) & 63.87 (0.72) & 20.10 (1.05) \\
        \noalign{\vskip 1mm}
        \cdashline{2-7}
        \noalign{\vskip 1mm}
        & Simod & 0.04 (0.00) & 0.07 (0.00) & 16.04 (0.00) & \textbf{1.09} (0.00) & \textbf{0.08} (0.00)\\
        & DSim & 0.12 (0.02) & NA & 21.44 (14.28) & 5.39 (5.80) & 7.39 (15.6) \\
        & ASim & \textbf{0.00} (0.02) & \textbf{0.04} (0.01) & \textbf{16.00} (7.94) & 2.04 (1.29) & 4.44 (6.78) \\   
        \midrule
        \multirow{4}{*}{\rotatebox{90}{C.1000}} & real & 0.71 (0.02) & 0.39 (0.00) & 21.23 (0.06) & 0.25 (0.00) & 0.41 (0.05) \\
        \noalign{\vskip 1mm}
        \cdashline{2-7}
        \noalign{\vskip 1mm}
        & Simod & 0.13 (0.01) & \textbf{0.00} (0.00) & 0.69 (0.47) & 1.09 (0.25) & 3.34 (2.52) \\
        & DSim & 0.48 (0.01) & NA & 5.67 (4.58) & 0.16 (0.07) & 0.04 (0.08) \\
        & ASim & \textbf{0.01} (0.02) & \textbf{0.00} (0.00) & \textbf{0.03} (0.04) & \textbf{0.02} (0.02) & \textbf{0.02} (0.06) \\        
        \midrule
        \multirow{4}{*}{\rotatebox{90}{C.2000}} & real &  0.71 (0.02) & 0.39 (0.00) & 21.44 (0.18) & 0.21 (0.00) & 0.38 (0.06) \\
        \noalign{\vskip 1mm}
        \cdashline{2-7}
        \noalign{\vskip 1mm}
        & Simod & 0.12 (0.01) & \textbf{0.00} (0.00) & 0.67 (0.31) & 1.47 (0.42) &  2.04 (2.41)\\
        & DSim & 0.50 (0.01) & NA & 3.29 (3.23) & 0.30 (0.09) & 1.65 (2.70) \\
        & ASim & \textbf{0.01} (0.03) & \textbf{0.00} (0.00) & \textbf{0.08} (0.09) & \textbf{0.01} (0.01) &  \textbf{0.02} (0.04)\\       
        \midrule        
        \multirow{4}{*}{\rotatebox{90}{CVS}} & real & 0.80 (0.03) & 0.94 (0.03) & 3.21 (0.06) & 25.36 (0.01) & 4.71 (0.01) \\
        \noalign{\vskip 1mm}
        \cdashline{2-7}
        \noalign{\vskip 1mm}
        & Simod & 0.30 (0.01) & 0.54 (0.08) & \textbf{0.00} (0.06) & 1.69 (0.24) & 2.02 (0.22) \\
        & DSim & 0.09 (0.01) & NA & 0.04 (0.02) & 29.89 (9.28) & 3.93 (2.57) \\
        & ASim & \textbf{0.02} (0.00) & \textbf{0.01} (0.00) & 0.06 (0.00) & \textbf{0.12} (0.06) & \textbf{0.10} (0.05) \\
        \midrule
        \multirow{4}{*}{\rotatebox{90}{Production}} & real & 0.54 (0.02) & 0.59 (0.02) & 120.00 (0.38) & 9.32 (0.29) &  5.75 (3.39)\\
        \noalign{\vskip 1mm}
        \cdashline{2-7}
        \noalign{\vskip 1mm}
        & Simod & 0.11 (0.03) & \textbf{0.14} (0.01) & 24.85 (10.37) & 41.50 (2.76) &  \textbf{0.05} (4.56)\\
        & DSim & 0.43 (0.07) & NA & \textbf{12.30} (6.06) & \textbf{9.21} (1.54) & 182.1 (112.90) \\
        & ASim & \textbf{0.00} (0.02) & 0.21 (0.07) & 27.87 (5.33) & 36.82 (2.95) & 2.93 (0.50) \\
        \midrule
        \multirow{4}{*}{\rotatebox{90}{CDM}} & real & 0.75 (0.02) & 0.68 (0.04) & 4.25 (0.13) & 12.31 (0.20) & 2.20 (0.02)\\
        \noalign{\vskip 1mm}
        \cdashline{2-7}
        \noalign{\vskip 1mm}
        & Simod & 0.27 (0.06) & 0.27 (0.04) & 0.49 (0.70) & 1.60 (1.00) & 0.11 (0.20) \\
        & DSim & 0.39 (0.08) & NA & 0.21 (0.18) & \textbf{0.10} (0.12) & \textbf{0.01} (0.02) \\
        & ASim & \textbf{0.13} (0.03) & \textbf{0.20} (0.07) & \textbf{0.04} (0.08) & 0.11 (0.06) & 0.01 (0.01) \\
        \midrule
        \multirow{4}{*}{\rotatebox{90}{BPI12W}} & real & 0.59 (0.06) & 0.75 (0.00) & 8.63 (0.13) & 26.53 (0.13) & 6.42 (0.94) \\
        \noalign{\vskip 1mm}
        \cdashline{2-7}
        \noalign{\vskip 1mm}
        & Simod & 0.38 (0.00) & \textbf{0.00} (0.00) & 0.21 (0.00) & 0.04 (0.00) & 0.20 (0.00) \\
        & DSim & 0.41 (0.02) & NA & 0.10 (0.05) & 0.05 (0.01) & \textbf{0.18} (0.03) \\
        & ASim & \textbf{0.02} (0.01) & \textbf{0.00} (0.00) & \textbf{0.04} (0.10) & \textbf{0.00} (0.11) & 0.21 (1.78) \\
        \midrule
        \multirow{4}{*}{\rotatebox{90}{BPI17W}} & real & 0.54 (0.01) & 0.88 (0.00) & 6.10 (0.55) & 33.01 (0.15) & 6.61 (0.40) \\
        \noalign{\vskip 1mm}
        \cdashline{2-7}
        \noalign{\vskip 1mm}
        & Simod & 0.23 (0.00) & 0.35 (0.00) & \textbf{0.56} (0.00) & 0.12 (0.00) & 0.68 (0.00) \\
        & DSim & 0.19 (0.02) & NA & 3.46 (3.66) & 0.10 (0.04) & 0.62 (0.06) \\
        & ASim & \textbf{0.08} (0.09) & \textbf{0.00} (0.00) & 1.70 (2.50) & \textbf{0.00} (0.15) & \textbf{0.25} (0.36) \\ 
        \bottomrule
    \end{tabular}
    \label{tab:results_LSTM}
\end{table}
\vspace*{\fill}

% Second full-page table without page number/style
\vspace*{\fill}
\begin{table}[htbp]
    \centering
    \caption{Performance of Transformer model on real and simulated data. Each table entry shows the average performance over 10 runs, with the standard deviation in parentheses.}
    \begin{tabular}{clrrrrr}
        \toprule
        Log & Data & NAP & NRP & NPP(min) & NWP(hour) & RTP(day) \\
        \midrule
        \multirow{4}{*}{\rotatebox{90}{P2P}} & real & 0.85 (0.01) & 0.88 (0.01) & 63.97 (3.26) & 61.88 (0.79) & 15.50 (0.22) \\
        \noalign{\vskip 1mm}
        \cdashline{2-7}
        \noalign{\vskip 1mm}
        & Simod & 0.02 (0.00) & \textbf{0.66} (0.00) & 114.22 (0.00) & \textbf{5.80} (0.00) & 2.96 (0.00) \\
        & DSim & 0.15 (0.03) & NA & 81.48 (89.20) & 6.86 (3.28) & 5.91 (4.05)\\
        & ASim & \textbf{0.00} (0.02) & \textbf{0.66} (0.04) & \textbf{17.21} (2.81) & 17.45 (3.84) & \textbf{1.66} (1.06) \\ 
        \midrule
        \multirow{4}{*}{\rotatebox{90}{C.1000}} & real & 0.74 (0.00) & 0.49 (0.01) & 17.06 (0.23) & 0.31 (0.01) & 0.36 (0.00) \\
        \noalign{\vskip 1mm}
        \cdashline{2-7}
        \noalign{\vskip 1mm}
        & Simod & 0.32 (0.02) & \textbf{0.12} (0.03) & \textbf{4.97} (034) & 3.05 (0.54) & 3.72 (0.44)\\
        & DSim & 0.55 (0.06) & NA & 7.22 (1.11) & \textbf{0.21} (0.01) & \textbf{0.10} (0.03)\\
        & ASim & \textbf{0.26} (0.02) & 0.18 (0.03) & 5.27 (0.56) & 0.37 (0.08) & 0.32 (0.07) \\
        \midrule
        \multirow{4}{*}{\rotatebox{90}{C.2000}} & real & 0.74 (0.00) & 0.54 (0.01) & 17.16 (0.41) & 0.28 (0.01) & 0.31 (0.01) \\
        \noalign{\vskip 1mm}
        \cdashline{2-7}
        \noalign{\vskip 1mm}
        & Simod & 0.28 (0.02) & \textbf{0.13} (0.05) & 4.98 (1.15) & 2.33 (0.35) & 3.11 (0.36)\\
        & DSim & 0.56 (0.05) & NA & 8.21 (1.16) & 0.38 (0.06) & \textbf{0.06} (0.04)\\
        & ASim & \textbf{0.19} (0.02) & 0.16 (0.13) & \textbf{4.89} (0.45) & \textbf{0.30} (0.07) & 0.21 (0.04) \\ 
        \midrule        
        \multirow{4}{*}{\rotatebox{90}{CVS}} & real & 0.72 (0.00) & 0.65 (0.00) & 3.32 (0.14) & 15.27 (0.50) & 1.61 (0.09) \\
        \noalign{\vskip 1mm}
        \cdashline{2-7}
        \noalign{\vskip 1mm}
        & Simod & 0.23 (0.01) & 0.65 (0.00) & 0.57 (0.33) & \textbf{27.57} (3.33) & 32.19 (1.88) \\
        & DSim & 0.19 (0.02) & NA & 0.61 (0.42) & 33.78 (10.22) & 15.82 (1.42)\\
        & ASim & \textbf{0.07} (0.01) & \textbf{0.06 (0.03)} & \textbf{0.12} (0.02) & 28.21 (4.82) & \textbf{1.18} (0.01) \\
        \midrule
        \multirow{4}{*}{\rotatebox{90}{Production}} & real & 0.59 (0.02) & 0.40 (0.04) & 121.66 (3.44) & 15.58 (1.69) & 10.61 (0.83) \\
        \noalign{\vskip 1mm}
        \cdashline{2-7}
        \noalign{\vskip 1mm}
        & Simod & 0.56 (0.02) & 0.31 (0.04) & 44.64 (53.96) & 12.73 (19.05) &  3.72 (20.12)\\
        & DSim & 0.48 (0.06) & NA & 12.11 (7.43) & 7.28 (1.21) & \textbf{0.05} (4.80)\\
        & ASim & \textbf{0.04} (0.02) & \textbf{0.01} (0.04) & \textbf{5.50} (2.70) & \textbf{5.06} (0.11) & 4.85 (0.99) \\
        \midrule 
        \multirow{4}{*}{\rotatebox{90}{CDM}} & real & 0.72 (0.00) & 0.55 (0.04) & 9.55 (0.83) & 8.58 (0.77) &  3.62 (0.13)\\
        \noalign{\vskip 1mm}
        \cdashline{2-7}
        \noalign{\vskip 1mm}
        & Simod & \textbf{0.16} (0.04) & \textbf{0.31} (0.13) & 2.00 (1.22) & 25.61 (3.50) & 10.65 (0.60)\\
        & DSim & 0.51 (0.07) & NA & \textbf{0.46} (0.83) & 10.36 (1.39) & \textbf{0.64} (0.26)\\
        & ASim & 0.17 (0.02) & 0.48 (0.15) & 0.48 (2.03) & \textbf{6.17} (0.23) & 1.44 (0.02) \\   
        \midrule
        \multirow{4}{*}{\rotatebox{90}{BPI12W}} & real & 0.76 (0.00) & 0.86 (0.00) & 9.00 (0.20) & 29.59 (0.30) & 4.81 (0.10) \\
        \noalign{\vskip 1mm}
        \cdashline{2-7}
        \noalign{\vskip 1mm}
        & Simod & 0.48 (0.00) & 0.02 (0.00) & \textbf{0.31} (0.00) & 17.50 (0.00) & 0.65 (0.00) \\
        & DSim & 0.47 (0.02) & NA & 1.90 (0.70) & 4.45 (1.50) & 2.08 (0.36)\\
        & ASim & \textbf{0.00} (0.01) & \textbf{0.01} (0.00) & 0.50 (0.09) & \textbf{0.38} (0.21) & \textbf{0.18} (0.04) \\        
        \midrule
        \multirow{4}{*}{\rotatebox{90}{BPI17W}} & real & 0.62 (0.01) & 0.99 (0.00) & 6.14 (0.26) & 33.23 (0.43) & 5.80 (0.06) \\ 
        \noalign{\vskip 1mm}
        \cdashline{2-7}   
        \noalign{\vskip 1mm}
        & Simod & 0.20 (0.00) & \textbf{0.00} (0.00) & 0.25 (0.00) & 9.48 (0.00) & \textbf{0.70} (0.00) \\
        & DSim & 0.29 (0.09) & NA & 0.07 (0.22) & 21.95 (12.02) & 8.08 (2.83)\\
        & ASim & \textbf{0.12} (0.14) & 0.16 (0.14) & \textbf{0.06} (0.08) & \textbf{9.22} (7.19) & 3.10 (4.28)\\
        \bottomrule
    \end{tabular}
    \label{tab:results_transformer}
\end{table}
\vspace*{\fill}

% Appendix bibliography explicitly AFTER both tables
\newpage
\bibliographystyleA{splncs04}
\bibliographyA{appendixbib}
